# Supplementary material for: MambaVO: Deep Visual Odometry Based on Sequential Matching Refinement and Training Smoothing
Source: arXiv:2412.20082 source file (2025-04-07)
Supplement: Supplementary file 1 [file X_suppl.tex]

\clearpage
\setcounter{page}{1}
\maketitlesupplementary
\appendix

\section{Implementation Details}
\label{supple:implement}

\subsection{Geometric Initialization Module}
\label{supple:GIM}

The images are resized to 448x224. Metric3D only runs once per keyframe.
We use pretrained EfficientLoFTR \cite{wang2024efficient} with mixed precision in the Geometric Initialization Module (GIM) to obtain initial matches. EfficientLoFTR performs both coarse and fine-level matching. The fine-level stage provides pixel-level correspondences along with their features, which serve as our initial matches and geometric features. Since semi-dense matching can produce numerous matching pixels per frame, we randomly select 100 matches per frame for subsequent pose estimation.

We employ the lightweight small version of Dino-v2 \cite{oquab2023dinov2} to generate generalized and robust semantic features. 
Specifically, we adopt the small version with registers as the pretrained weights of Dino-v2 model.
For each input frame, Dino-v2 produces patch-level features with 384 channels. These patch features are reorganized and deconvolved to the pixel level to obtain semantic features for each pixel. Using the initial matching coordinates, the corresponding semantic features are queried and fused with geometric features to form the matching feature (\cref{sec:initialization}). The resulting matching feature is then fed into the Geometric Mamba Module.

\subsection{Geometric Mamba Module}

\begin{figure}[ht]
  \centering
  \includegraphics[width=0.95\linewidth]{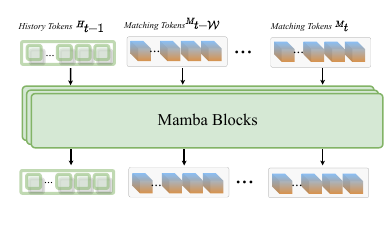}
  \caption{Illustration of Mamba blocks in Geometric Mamba Module. }
  \label{fig:mamba}
\end{figure}

In the Geometric Mamba Module, we set the number of Mamba blocks $B$ to 3. The input to Mamba at frame $t$ consists of the history tokens from frame $t-1$ and all matching tokens of frames $t-\mathcal{W}$ to $t$, in chronological order. 
Mamba blocks output updated history tokens and matching tokens.

This design of input leverages Mamba's long-distance modeling capabilities, utilizing historical interactions to adjust matching tokens and estimate the refinement and weight of each matching pixel.

\section{Qualitative Results}

\subsection{Matching Comparison}

The accuracy of visual odometry heavily depends on computing visual correspondences between frames. In MambaVO, we first use semi-dense matching for initial correspondences, then refine them using the Mamba architecture with temporal information. Experimental results demonstrate that our matching approach outperforms previous visual odometry methods in terms of pose accuracy between frames (\cref{sec:matching}).

To intuitively demonstrate the matching quality of MambaVO, we visualize the matching pixels of MambaVO and the previous SOTA method DPVO \cite{teed2024deep} in \cref{fig:matching}. DPVO initializes 96 patches for matching per frame. During visualization, we remove invalid matches (those beyond the image coordinate range) and mark only the center points for clarity.

Compared to DPVO, which often produces ambiguous, inaccurate matches, MambaVO delivers more accurate, consistent, and evenly distributed matching points on the image plane, benefiting subsequent pose estimation.

\subsection{Trajectory and Map Visualization}

We visualize the results of MambaVO++ on EuRoC \cite{burri2016euroc}, TartanAir \cite{wang2020tartanair}, KITTI \cite{geiger2012we} and TUM-RGBD \cite{sturm12iros} and the trajectories are illustrated in \cref{fig:tra1} and \cref{fig:tra2} respectively. The sparse maps are visualized in \cref{fig:map}.

Among the four datasets, TartanAir is a simulation dataset, while the other three are collected from real-world environments. TartanAir covers both indoor and outdoor scenes, with trajectories ranging from a few meters to several tens of meters.
The EuRoC dataset, collected by drones in indoor environments, shows that our method's results align closely with the ground truth in most sequences.
TUM-RGBD is a challenging indoor dataset characterized by erratic camera motion and significant motion blur. As seen in the experimental results (\cref{tab:tum}) and trajectory plots (\cref{fig:tra2}), our method remains effective under these demanding conditions.
KITTI, an outdoor autonomous driving dataset, typically features large-scale, high-speed movements. To evaluate our method's performance on long-distance scenarios, we selected five sequences, including both those with and without loop closures, as in \cref{fig:tra2}.

\section{Additional Experiments}
\subsection{Architecture Comparison}
To further verify the rationality of the Mamba architecture, we conduct a comparative experiment between the Mamba and Transformer architectures. We replace Mamba with Transformer and the result is shown \cref{tab:transformer}.
Mamba is, light-weight, computationally efficient,  and produces more accurate results.
\begin{table}[h]
\centering
\begin{tabular}{c|cc}
\toprule
Dataset      & \multicolumn{2}{c}{EuRoC}  \\ 
Metirc       & ATE$\downarrow$         & FPS$\uparrow$             \\ \midrule
TransfomerVO & 0.112       & 17Hz               \\
MambaVO      & \textbf{0.094}& \textbf{22Hz}    \\ \bottomrule
\end{tabular}
\caption{Comparative experiment between Mamba architecture and Transformer architecture.}
\label{tab:transformer}
\end{table} 

\subsection{Time Analysis}
We have made a lot of efforts to try to improve the efficiency of our system (\cref{supple:implement}). Following other SLAM methods (TartanVO, DROID-SLAM, DPVO), we skip every other frame, as consecutive frames have similar images and poses. This nearly doubles the frame rate. We evaluate the average per-frame time (ms) on EuRoC (\cref{tab:time}).
\begin{table}[H]
\centering
\scalebox{0.72}{
\begin{tabular}{@{}c|c@{\hspace{0.5em}}c@{\hspace{0.5em}}c@{\hspace{0.5em}}c@{\hspace{0.5em}}c@{\hspace{0.5em}}c@{\hspace{0.5em}}c}
\toprule
Module    & E-LoFTR & Metric3D & DINO-v2 & PnP  & cross-attention & Mamba & BA \\ \midrule
Avg. time$\dagger$ & 14.2    &  18.3    & 28.8    & 11.6 & 3.1             & 12.0    & 11.7  \\ 
Avg. time$\ast$& 7.1     &  3.5     & 14.4    & 5.8  & 1.55            & 6.0     & 5.85   \\ \bottomrule
\end{tabular}}
\caption{The average time for each part of MambaVO on EuRoC.}
\label{tab:time}
\end{table}
\noindent\footnotesize $\dagger$ indicates the running time it takes for the module to process one image. $\ast$ represents the total time of each module of a trajectory divided by the number of frames, which represents the actual average rates.

\normalsize 
\section{Limitations}
Our proposed MambaVO can only obtain sparse maps because only semi-dense matching pixels in GIM are used to build the map. In the future, we will utilize dense information and 3D Gaussian Splatting \cite{kerbl20233d} technology to obtain high-fidelity maps for rich scene representation while maintaining localization accuracy.

\begin{figure*}[ht]
  \centering
  \includegraphics[width=0.89\linewidth]{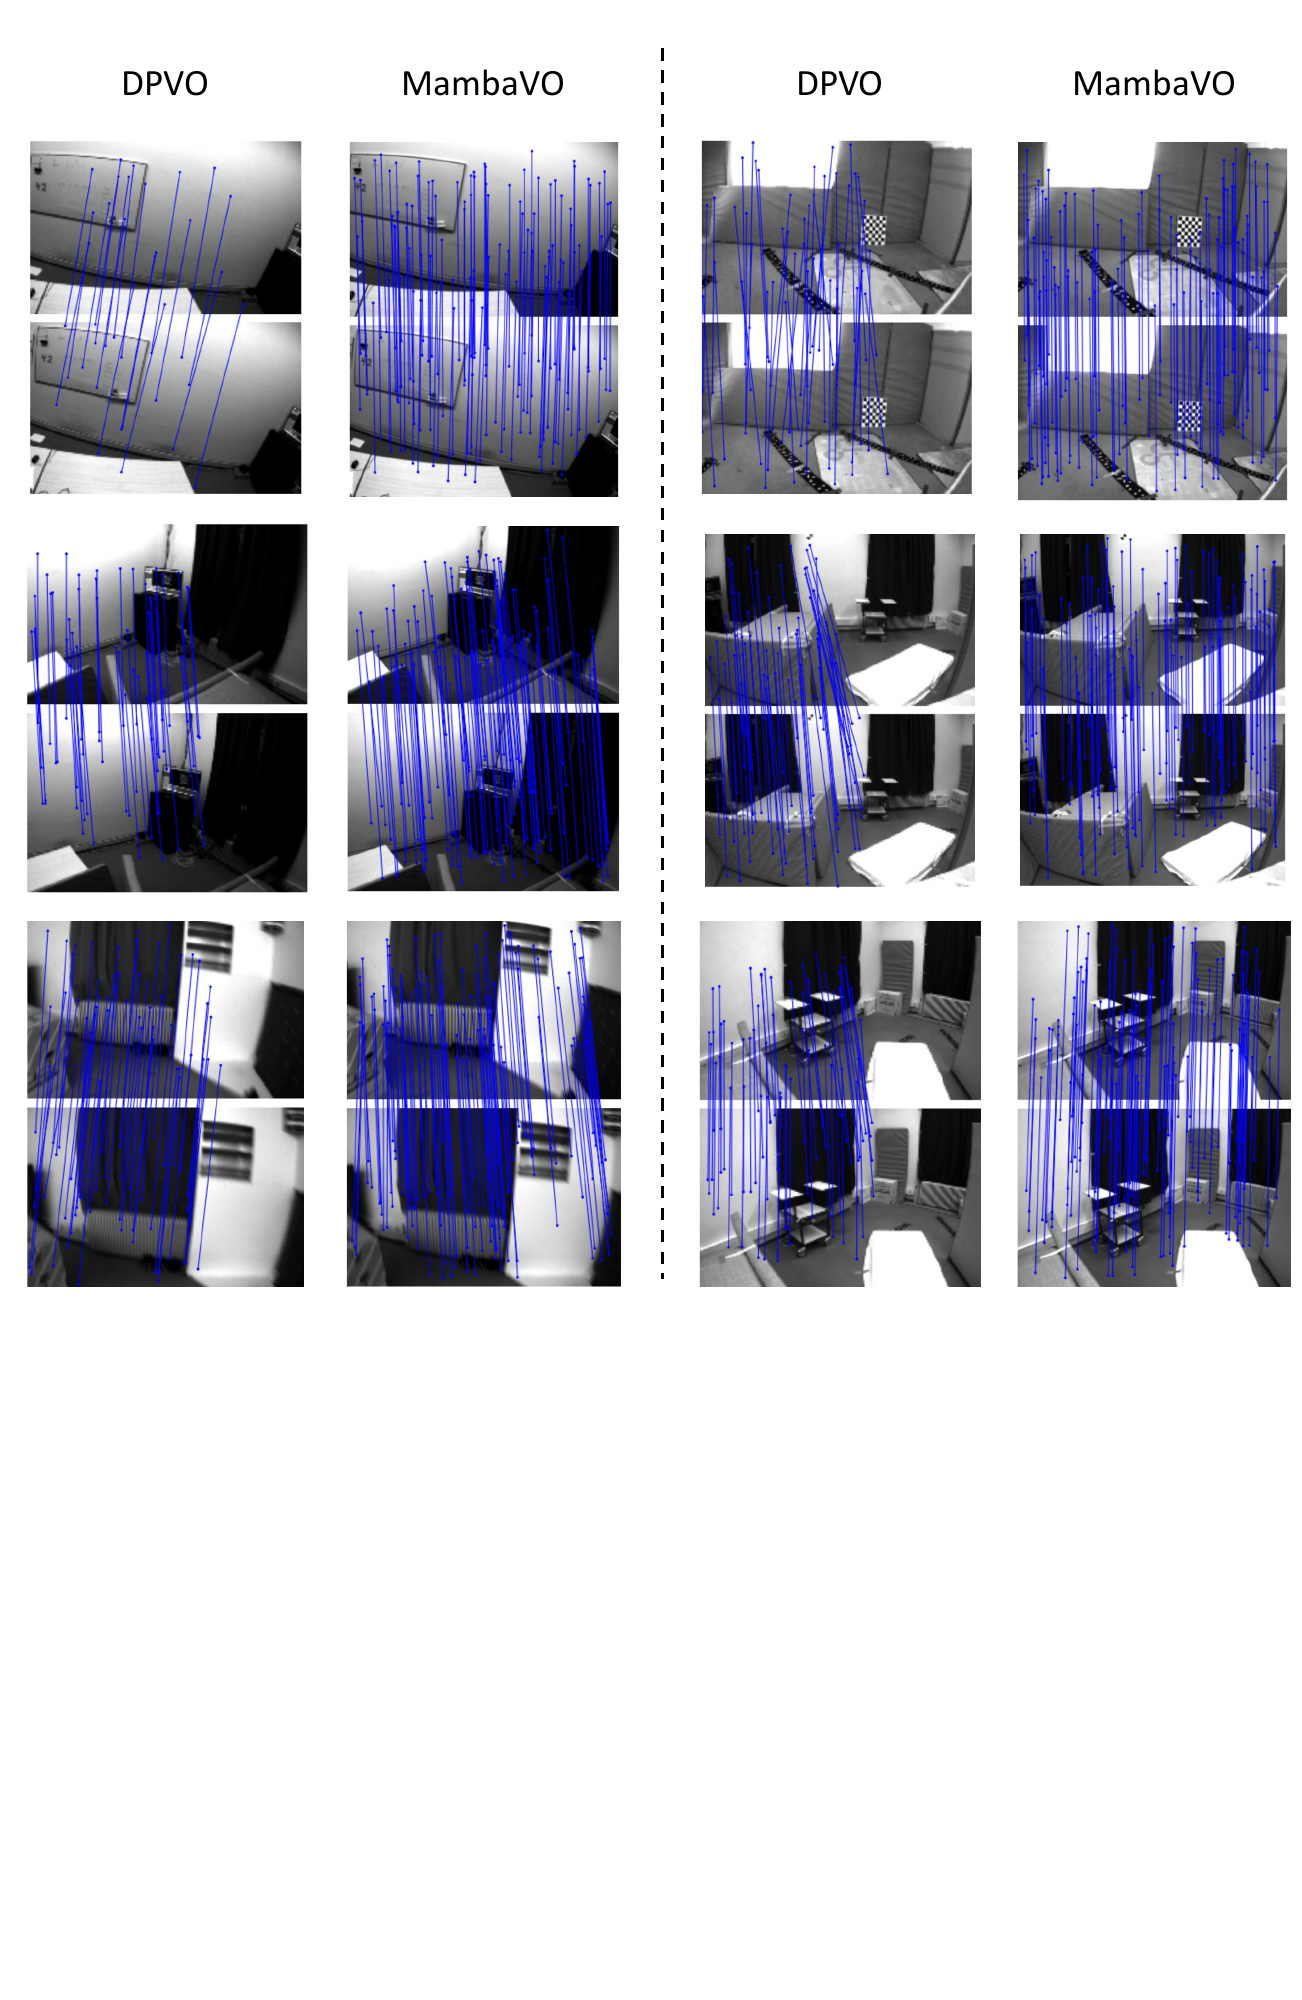}
  \caption{Matching results of two consecutive frames in DPVO and MambaVO. The matching quality of MambaVO, including accuracy and distribution, is better than DPVO \cite{teed2024deep}, which is the previous SOTA deep visual odometry.}
  \label{fig:matching}
\end{figure*}

\begin{figure*}[ht]
  \centering
  \includegraphics[width=0.67\linewidth]{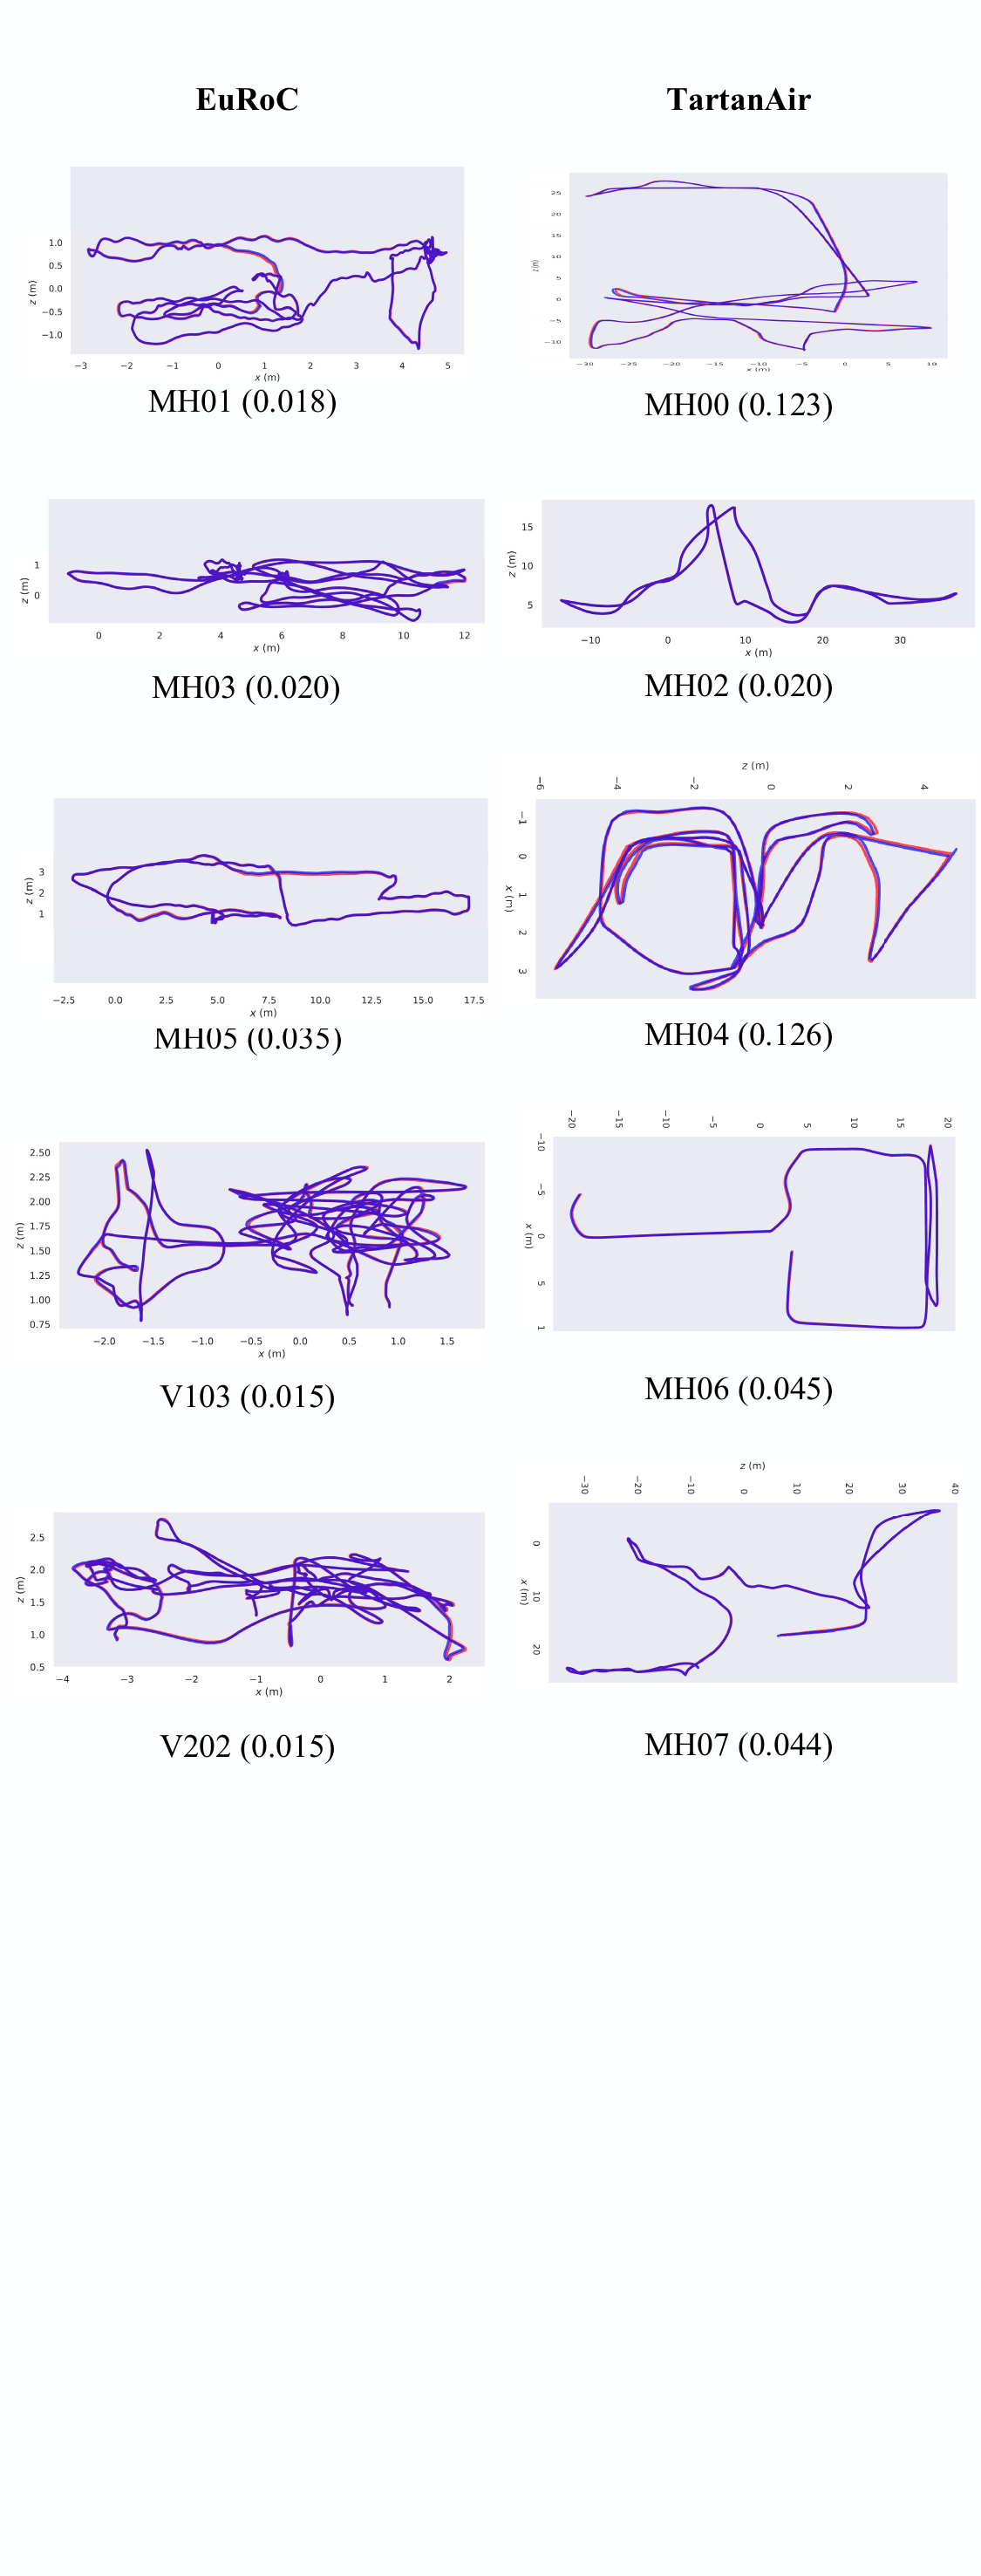}
  \caption{Qualitative visualization of MambaVO++ on EuRoC and TartanAir. The blue line represents the trajectory estimated by MambaVO++, and the red line represents the ground truth. The results show that our estimated trajectory almost completely coincides with the ground truth.}
  \label{fig:tra1}
\end{figure*}

\begin{figure*}[ht]
  \centering
  \includegraphics[width=0.69\linewidth]{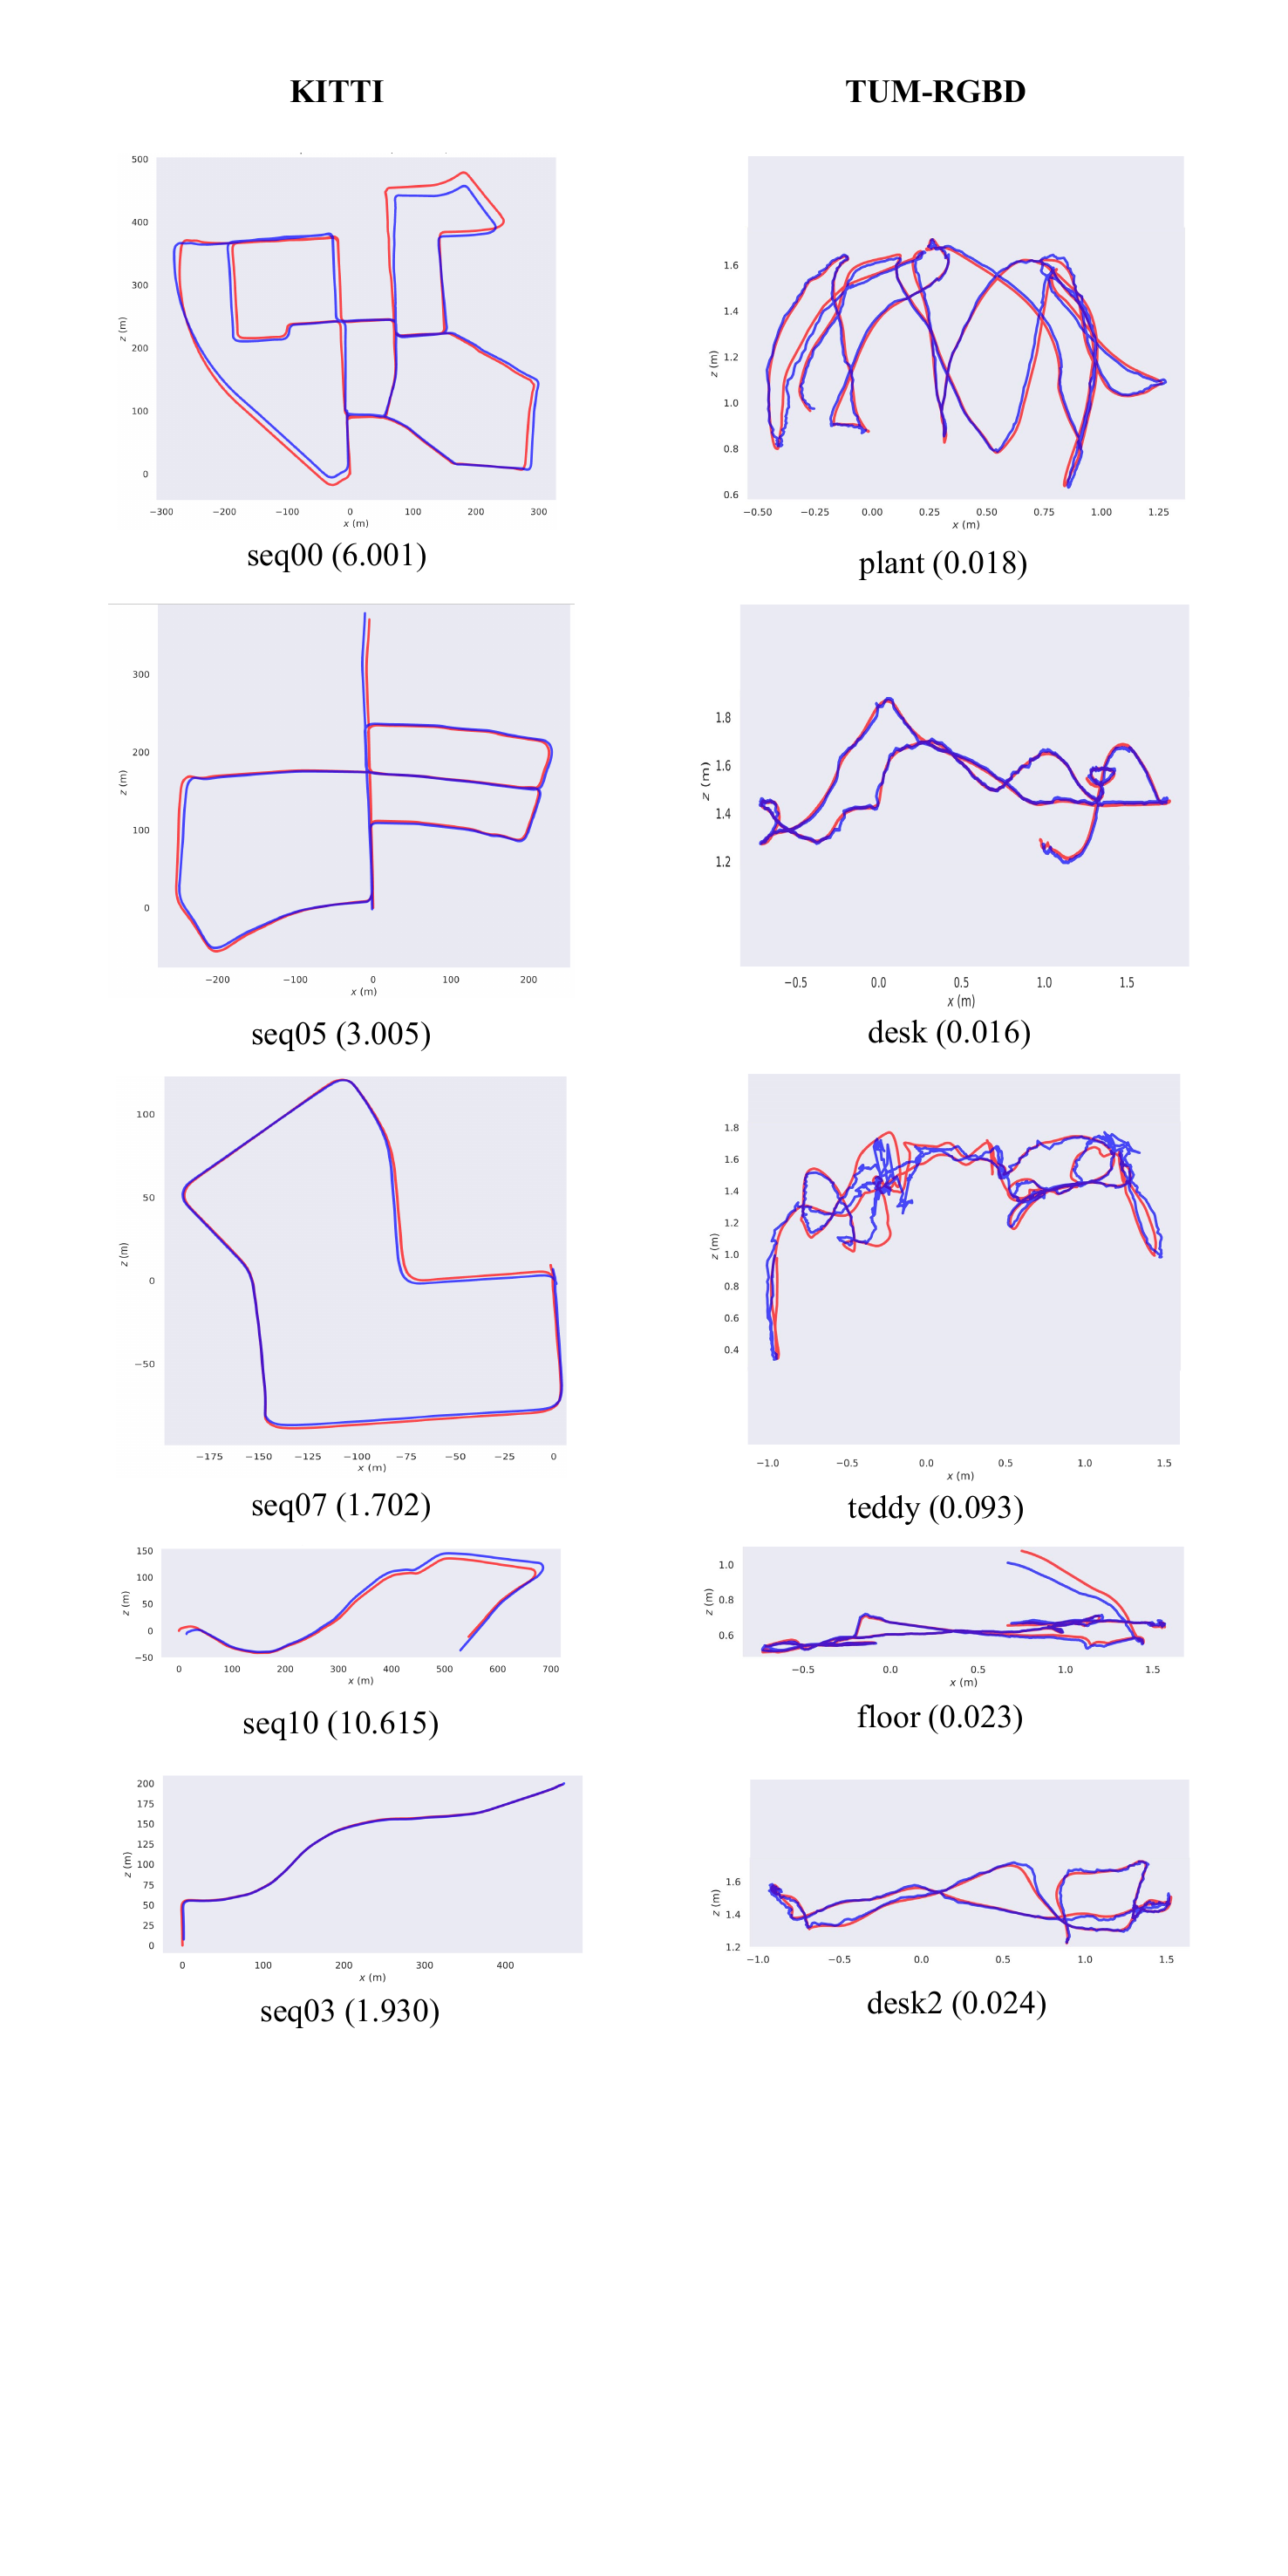}
  \caption{Qualitative visualization of MambaVO++ on KITTI and TUM-RGBD. The blue line represents the trajectory estimated by MambaVO++, and the red line represents the ground truth. The results show that our estimated trajectory almost completely coincides with the ground truth.}
  \label{fig:tra2}
\end{figure*}

\begin{figure*}[ht!]
    \centering
    \begin{subfigure}[b]{0.45\textwidth}
        \centering
        \includegraphics[width=0.8\textwidth]{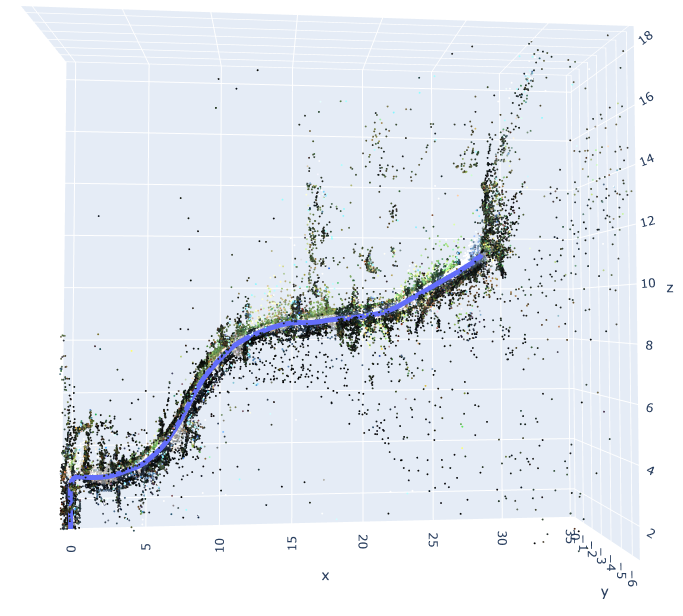} 
        \caption{}
        \label{fig:sub1}
    \end{subfigure}
    \hspace{5mm}
    \begin{subfigure}[b]{0.45\textwidth}
        \centering
        \includegraphics[width=0.8\textwidth]{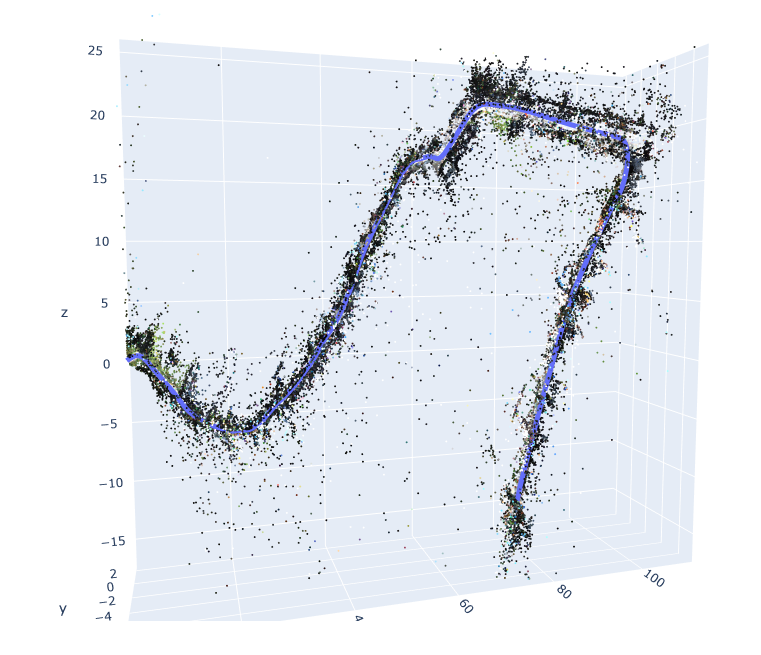}
        \caption{}
        \label{fig:sub2}
    \end{subfigure}
    \vspace{1mm}
    \begin{subfigure}[b]{0.45\textwidth}
        \centering
        \includegraphics[width=0.8\textwidth]{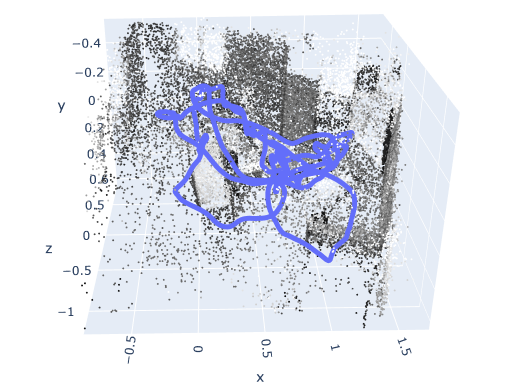}
        \caption{}
        \label{fig:sub3}
    \end{subfigure}
    \hspace{5mm}
    \begin{subfigure}[b]{0.45\textwidth}
        \centering
        \includegraphics[width=0.8\textwidth]{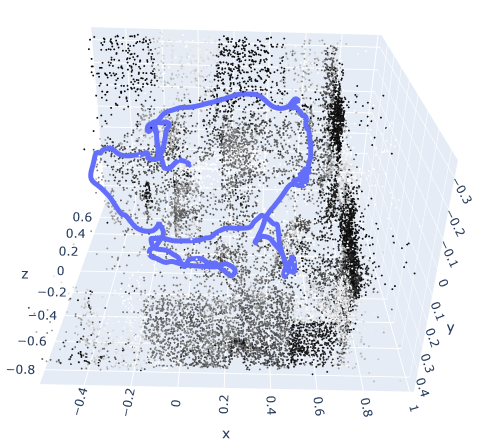}
        \caption{}
        \label{fig:sub4}
    \end{subfigure}
    \caption{The proposed MambaVO can produce trajectories and sparse maps. We visualize the trajectories and sparse maps of KITTI (a and b) and EuRoC (c and d) respectively. The blue line represents the trajectories and the points respresent the map points.
}
    \label{fig:map}
\end{figure*}
